# Supplementary material for: Few-Shot Physically-Aware Articulated Mesh Generation via Hierarchical Deformation
Source: arXiv:2308.10898 source file (2023-08-21)
Supplement: Supplementary file 1 [file supp.tex]

\begin{table*}[t]
    \centering
    \caption{\footnotesize 
    Comparison between the performance of each method for articulated object generation on all categories. 
    MMD is multiplied by $10^3$ and APD is multiplied by $10^2$.
    \textbf{Bold} for best values. 
    } 
    \begin{tabular}{@{\;}c@{\;}|c|c|c|c|c|c|c|c@{\;}}
    \midrule
        \hline
        \specialrule{0em}{1pt}{0pt} 
        ~ & Method & \makecell[c]{Storage\\ Furniture} & Scissors &  Eyeglasses  & Oven & Lamp & TrashCan & Avg. \\ 
        \cline{1-9} 
        \specialrule{0em}{1pt}{0pt}
        
        % mean error / Median error
        \multirow{3}{*}{MMD~($\downarrow$)} & MetaHandles w/ Obj. & 1.097 & 3.336 &8.336 & 7.611 & 12.191 & 9.307 & 6.980
        \\ \cline{2-9} 
        \specialrule{0em}{1pt}{0pt}
        
        ~  & Ours w/0 Hier. & 2.001 & 4.115 & 8.930 & 7.203 & 11.993 & 8.781 & 7.170
        \\ \cline{2-9} 
        \specialrule{0em}{1pt}{0pt}

        % ~ & Ours w/o TTA & - & 1.291 & 6.212 & - & - & - & -  
        % \\ \cline{2-9} 
        % \specialrule{0em}{1pt}{0pt}

        ~ & Ours w/o transfer & 1.066 & 1.923 & 6.211 & 7.124 & 7.451 & 8.772 & 5.424
        \\ \cline{2-9} 
        \specialrule{0em}{1pt}{0pt}

        ~ & Ours w/ transfer & 1.058 & 1.495 & 6.062 & 7.009 & 7.133 & 8.430  & 5.198
        \\ \cline{1-9} 
        \specialrule{0em}{1pt}{0pt}

        % mean error / Median error
        \multirow{3}{*}{COV~(\%, $\uparrow$)} & MetaHandles w/ Obj. & 43.07 & 33.49 & 19.51 & 60.00 & 50.00 & 17.14 & 37.20
        \\ \cline{2-9} 
        \specialrule{0em}{1pt}{0pt}

         ~ & Ours w/0 Hier. & 39.35 & 33.66 & 18.33 & 60.00  & 50.00 & 17.14 & 36.41
        \\ \cline{2-9} 
        \specialrule{0em}{1pt}{0pt}
        
        % ~ & Ours w/o TTA  & - & 55.34 & 29.82 & - & - & - & - 
        % \\ \cline{2-9} 
        % \specialrule{0em}{1pt}{0pt}

        ~ & Ours w/o transfer  & 73.08 & 48.78 & 18.33 & 60.00 & 62.50 & 17.14 & 46.64
        \\ \cline{2-9} 
        \specialrule{0em}{1pt}{0pt}

        ~ & Ours w/ transfer & 75.33 & 57.89 & 29.82 & 60.00 & 62.50 & 17.14 & 50.45
        \\ \cline{1-9} 
        \specialrule{0em}{1pt}{0pt}

        % mean error / Median error
        \multirow{3}{*}{1-NNA~(\%, $\downarrow$)} & MetaHandles w/ Obj. & 97.97 & 98.18 & 98.43 & 98.17 & 95.33 & 86.05 & 95.69
        \\ \cline{2-9} 
        \specialrule{0em}{1pt}{0pt}

        % ~ &  Ours w/o TTA & - & 96.04  & 98.57 & - & - & - & - 
        % \\ \cline{2-9} 
        % \specialrule{0em}{1pt}{0pt}

        ~ & Ours w/o Hier.  & 98.66 & 97.13 & 98.34 & 97.47 & 98.20 & 82.78 & 95.43
        \\ \cline{2-9} 
        \specialrule{0em}{1pt}{0pt}

        ~ &  Ours w/o transfer & 98.69 & 96.39 & 96.69 & 97.56 & 93.41 & 75.33 & 93.01
        \\ \cline{2-9} 
        \specialrule{0em}{1pt}{0pt}

        ~ &  Ours w/ transfer & 97.76 & 97.02  & 98.26 & 96.59 & 92.44 & 72.09 & 92.36
        \\ \cline{1-9} 
        \specialrule{0em}{1pt}{0pt}

        % mean error / Median error
        \multirow{3}{*}{JSD~($\downarrow$)} & MetaHandles w/ Obj. & 0.0626 & 0.2119 & 0.0981 & 0.1694 & 0.1929 & 0.2171 & 0.1587
        \\ \cline{2-9} 
        \specialrule{0em}{1pt}{0pt}

         ~ & Ours w/o Hier. & 0.0630 & 0.1941 & 0.0800 & 0.1913 & 0.2132 & 0.1533 & 0.1492
         \\ \cline{2-9} 
        \specialrule{0em}{1pt}{0pt}
         
        % ~ & Ours w/o TTA & - & 0.1277 & 0.0757 & - & - & - & -  
        % \\ \cline{2-9} 
        % \specialrule{0em}{1pt}{0pt}

        ~ & Ours w/o transfer& 0.0297 & 0.1198 & 0.0766 & 0.1680 & 0.1911 & 0.1102 & 0.1159
        \\ \cline{2-9} 
        \specialrule{0em}{1pt}{0pt}

        ~ & Ours w/ transfer & 0.0290 & 0.1274 & 0.0681 & 0.1597 & 0.1874 & 0.0994 & 0.1118 
        \\ \cline{1-9} 
        \specialrule{0em}{1pt}{0pt}

        % mean error / Median error
        \multirow{2}{*}{APD~($\downarrow$)} & MetaHandles w/ Obj. & 0.1765 & 1.4280 & 0.1917 & 0.1640 & 7.384 & 0.0790 & 1.5705
        \\ \cline{2-9} 
        \specialrule{0em}{1pt}{0pt}

        % ~ & Ours w/o TTA & - & 1.381  & 0.1802 & - & - & - & - 
        % \\ \cline{1-9} 
        % \specialrule{0em}{1pt}{0pt}

        ~ & Ours w/o Hier. & 0.1839 & 1.6635  & 0.2042 & 0.1697 & 6.669 & 0.0881 & 1.4964 
        \\ \cline{2-9} 
        \specialrule{0em}{1pt}{0pt}

        ~ & Ours w/o transfer & 0.1700 & 1.5620  & 0.1740 & 0.1587 & 6.161 & 0.0680 & 1.3822 
        \\ \cline{2-9} 
        \specialrule{0em}{1pt}{0pt}

        ~ & Ours w/ transfer  & 0.1700 & 1.3520  & 0.1707 & 0.1602 & 5.993 & 0.0693 & 1.3192 
        \\ \cline{1-9} 
        \specialrule{0em}{1pt}{0pt}

    \end{tabular}
    % }
    % \vspace{-16pt}
    \label{tb_exp_gen_comparison_abl}
\end{table*}
