# Supplementary material for: Few-Shot Physically-Aware Articulated Mesh Generation via Hierarchical Deformation
Source: arXiv:2308.10898 source file (2023-08-21)
Supplement: Supplementary file 2 [file discussions.tex]

% !TEX root = ../supp.tex

\section{Discussions}

\begin{itemize}
    \item whts are common shape knowledge that can be transfer across categories
\end{itemize}
