# Supplementary material for: Few-Shot Physically-Aware Articulated Mesh Generation via Hierarchical Deformation
Source: arXiv:2308.10898 source file (2023-08-21)
Supplement: Supplementary file 3 [file method_old.tex]

% !TEX root = ../supp.tex

The document provides a list of supplemental materials to support the main paper: 
\begin{itemize}
    \item \textbf{Further Explanations on the Method -- }   We provide some additional explanations on our method for details that are not covered in the 
    % to illustrate details that are not covered in the 
    main paper (Sec.~\ref{sec_method_details_supp}), including
        \begin{itemize}
            \item \emph{Convex Deformation Synchronization} (Sec.~\ref{sec_supp_cvx_def}). We provide the 
            % a detailed 
            algorithm for the designed synchronization strategy. 
            \item \emph{Deformation Basis Optimization} (Sec.~\ref{sec_supp_def_basis}). We illustrate how we optimize the basis prediction network.
            \item \emph{Physically-aware Part Shape Composition} (Sec.~\ref{sec_supp_part_composition}). We further explain our collision avoidance strategy for part shape composition, namely the collision penalty term and the 
            % the collision penalty term and our 
            collision response-based deformation projection strategy. 
            \item \emph{Additional Explanations} (Sec.~\ref{sec_supp_method_additional_details}), including some other details such as convex decomposition and the mesh deformation smoothing strategy for part meshes. 
        \end{itemize}
    \item \textbf{Additional Experiments -- } We provide additional experiments to further validate the effectiveness of our method (Sec.~\ref{sec_supp_exp}), including
        \begin{itemize}
            \item \emph{Few-shot Mesh Generation} (Sec.~\ref{sec_supp_few_shot_mesh_gen}).  We further examine the few-shot generation ability of our hierarchical deformation strategy by testing it on different few-shot generation settings and also on rigid categories. 
            % its few-shot generation ability by testing the hierarchical deformation strategy on various few-shot generation settings and rigid categories . 
            \item \emph{Transfer Learning for Convex Deformations} (Sec.~\ref{sec_supp_tranfer_cvx_def}). We empirically demonstrate the superiority of convex-level deformation patterns transferring over the object-level trail. Moreover, we also explore the influence of source categories on the few-shot generation performance.  
            % of fine-tuned models. 
            \item \emph{Generation via Deformation} (Sec.~\ref{sec_supp_exp_gen_via_deform}). We discuss another approach to solve this problem not based on mesh deformations to explain why we choose mesh deformation as our underlying generation technique. 
            % We want to give 
            % By discussing its pros and cons, we give 
            % an answer to why we choose mesh deformation as our underlying generation technique. 
            \item \emph{Implementation Details} (Sec.~\ref{sec_supp_imp_details}). We provide the experimental settings. 
        \end{itemize}
\end{itemize}

We include a video to introduce our work in the supplementary material together with this document. 
We will release the code and data upon publication. 

\section{Method Details} \label{sec_method_details_supp}

% \begin{itemize}
%     \item detail of baseline strategies?
% \end{itemize}

% This section we aim to make some further clarifications on the proposed method, including the convex synchronization strategy, convex deformation basis optimization, loss functions, collision response-based projection strategy, and some additional details.
We provide some further explanations of the proposed method, including the convex deformation synchronization strategy, deformation basis optimization, collision avoidance strategy for physically-aware part shape composition, 
% collision response-based projection strategy, 
and some additional details.

\subsection{Convex Deformation Synchronization} \label{sec_supp_cvx_def}
Given each shape from a specific category $\mathcal{X}_i\in \mathcal{X}$, 
a set of  convex bases 
$\{ \mathbf{B}_i \vert 1\le i\le C \}$
, and their corresponding  coefficients 
$\{ \mathbf{A}_i \vert 1\le i\le C\}$ 
,  we wish to find a set of transformation matrices $\{ \mathbf{S}_i\in \mathbb{R}^{K\times K} \vert 1\le i\le C \}$ such that for each transformation, there exists a coefficient vector $\mathbf{a}\in \mathbb{R}^K$ same for all convexes and can transform each source shape to 
the original deformed shapes with the minimum average error, \emph{i.e.,}
\begin{align}
    [\{ \mathbf{S}_i \}, \{\mathbf{a}^j \}] = {\arg\min}_{[\{ \mathbf{S}_i \}, \{\mathbf{a}^j \}]} \sum_{j=1}^{\vert \mathcal{X}\vert} \sum_{i=1}^{C} \Vert \mathbf{B}_i\mathbf{S}_i\mathbf{a}^j - \mathbf{B}_i\mathbf{a}_i^j \Vert_2.  \label{eq_sync_supp}
\end{align} 
We adopt an iterative optimization strategy by looping: 
\begin{itemize}
    \item 1) Given a set of $\{ \mathbf{a}^j \}$, find $\mathbf{S}_i$ to optimize~\ref{eq_sync_supp}. 
    \item 2) Given a set of $\mathbf{S}_i$, find $\{ \mathbf{a}^j \}$ to optimize~\ref{eq_sync_supp}.  
\end{itemize}
Details of the optimization process is shown in Algorithm~\ref{algo_cvx_def_sync}. 

% A_i \in R^{K \times target shape}

\begin{algorithm}[H]
% \algsetup{linenosize=\tiny}
\small %\small, \footnotesize, \scriptsize, or \tiny
\caption{Convex deformation synchronization. 
% ``Average'' means computing an average vector of input vectors. 
``lsq'' means the least square solver. 
}
\label{algo_cvx_def_sync}
\footnotesize
    \begin{algorithmic}[1]
        \Require
            A set of convex bases $\{ \mathbf{B}_i \vert 1\le i\le C \}$, transformation coefficients $\{ \mathbf{A}_i \vert 1\le i\le C\}$, number of optimization iterations $T$. 
        \Ensure
            A set of transformation matrices $\{ \mathbf{S}_i\in \mathbb{R}^{K\times K} \vert 1\le i\le C \}$ , a set of transformation coefficients $\{\mathbf{a}^j \in \mathbb{R}^K \vert 1\le j \le \vert \mathcal{X} \vert \}$. 
        
        \State $\mathbf{a}^j \leftarrow \text{Average}(\mathbf{A}_1[j], ..., \mathbf{A}_C[j])$ % average of all coeffieicnets
        % \State $\mathcal{S}_{prev} \leftarrow \emptyset $
        \For{$t = 1$ to $T$}
            \For{$i \in [1, C]$}
            \State $\mathbf{A} \leftarrow \text{Stack}(\{ \mathbf{a}^j \}, \text{dim}=-1)$
            \State $\mathbf{A}_i \leftarrow \text{Stack}(\{ \mathbf{a}_i^j \}, \text{dim}=-1)$
            % \State SVD decomposition: $\mathbf{A} = \mathbf{U} \mathbf{\Sigma} \mathbf{V}^T$
            \State $[\mathbf{U}, \mathbf{\Sigma}, \mathbf{V}^T] \leftarrow \text{SVD}(\mathbf{A})$
            % \State SVD decomposition: $\mathbf{A}_i = \mathbf{U}_i \mathbf{\Sigma}_i \mathbf{V}_i^T$
            \State $[\mathbf{U}_i, \mathbf{\Sigma}_i, \mathbf{V}_i^T] \leftarrow \text{SVD}(\mathbf{A}_i)$
            \State $\mathbf{S}_i \leftarrow \mathbf{U}_i \mathbf{\Sigma}_i \mathbf{V}_i^T \mathbf{V} \mathbf{\Sigma}^+ \mathbf{U}^T$
            \EndFor

            
            \For{$j \in [1, \vert \mathcal{X} \vert ]$}
            \State $\mathcal{S}_{\mathbf{a}^j}\leftarrow \emptyset$
                \For{$i \in [1, C]$}
                \State $\hat{\mathbf{a}}_i^j\leftarrow \text{lsq}(\mathbf{S}_i, \mathbf{a}_i^j)$
                \State $\mathcal{S}_{\mathbf{a}^j} \leftarrow \mathcal{S}_{\mathbf{a}^j}  \cup \{ \hat{\mathbf{a}}_i^j \}$
                \EndFor
            \State $\mathbf{a}^j = \text{Average}(\mathcal{S}_{\mathbf{a}^j})$
            \EndFor
            
        \EndFor\\
        \Return $\{ \mathbf{S}_i \}$, $\{ \mathbf{a}^j \}$
        
    \end{algorithmic}
\end{algorithm}




\subsection{Deformation Basis Optimization} \label{sec_supp_def_basis}
% how to optimize basis, how to only
% basis prediction loss
For cage-based convex deformation, we represent the cage deformation as the linear combination of $K$ deformation bases, \emph{i.e.,} $\mathbf{B} = \{ \mathbf{b}_i\vert 1\le i\le K \}$, 
$\Delta \mathcal{C} = \sum_{i=1}^K a_i \mathbf{b}_i, a_i\in [0, 1], \forall 1\le i\le K$. 
We then use a network to learn a shape-dependent basis prediction function: 
\begin{equation}
    f_{\mathbf{B}}:   (\mathcal{X}_i \in \mathbb{R}^{N\times 3}, \mathcal{C} \in \mathbb{R}^{N_C\times 3}) \rightarrow \mathbf{B} \in \mathbb{R}^{K\times (N_C\times 3)}
\end{equation}
that maps the input shape and one of its convex 
% that maps the convex and shape points in the convex 
to a set of convex deformation bases. 
For a cage deformation $\Delta \mathcal{C}$, we optimize a set of coefficients $\mathbf{a} \in \mathbb{R}^{K\times 1}$ 
% of deformation bases 
to represent the deformation via predicted deformation bases $\mathbf{B}$, \emph{i.e.,} $\mathbf{a} = {\arg\min}_{\mathbf{a}} \Vert \mathbf{B}^T \mathbf{a} - \Delta \mathcal{C}\Vert_2$. 
The problem is solved via a least square solver, \emph{i.e.,} $\mathbf{a} = \text{lsq}(\mathbf{B}^T, \Delta \mathcal{C})$. 
Then, the cage basis prediction loss for matching vertex offsets is as follows: 
\begin{equation}
    \mathcal{L}_{offset} = \Vert  \mathbf{B}^T  \mathbf{a} - \Delta \mathcal{C} \Vert_2.  
\end{equation}
Besides, we add orthogonal and sparse losses for predicted deformation bases following~\cite{liu2021deepmetahandles}, denoted as $\mathcal{L}_{orth}$ and $\mathcal{L}_{sp}$ respectively. 
The total basis prediction loss is a linear combination of the above loss terms: $\mathcal{L}_{basis} = \mathcal{L}_{offset} + \lambda_{orth}\mathcal{L}_{orth} + \lambda_{sp} \mathcal{L}_{sp}$. 
$\lambda_{orth}$ and $\lambda_{sp}$ are hyperparameters. 
% \todo{orth loss and spare loss}


% \subsection{Physical losses}


\subsection{Physically-aware Part Shape Composition} \label{sec_supp_part_composition}
% To compose part shapes into the object, we design a collision penalty term and a collision response-based deformation projection strategy to guide the network towards physically-aware samples. 
We leverage a collision avoidance strategy when composing part shapes for an object. 
Its two main components are the collision penalty term and the collision response-based deformation projection. 
% There are two important losses in the 
% Two losses play an important role in the 
% physically-aware part composition process, namely the collision penalty term $\mathcal{L}_{phy}$ and the projection loss $\mathcal{L}_{proj}$. 
We will elaborate the details of the penalty term $\mathcal{L}_{phy}$  and the projection loss $\mathcal{L}_{proj}$ in the following text. 
% We will elaborate their details in the following text. 

$\mathcal{L}_{phy}$ use the penetration depth as the metric to measure collision and further add losses. 
$\mathcal{L}_{proj}$ points out the direction that collided mesh vertices should be projected to such that the collision penalty term could be reduced.
We provide their calculation details in Algorithm~\ref{algo_phy_sim}. 
We set $N_{step}$ to 100 and $N_{det}$ to 100. 
% \todo{add a algo for the physical simulation process and how we calculate the above losses}
% modify collided mesh vertices such that the collision penalty term 
% The 
% add penetration depth

\vpara{Average penetration depth.}
The value of the average penetration depth is the same to the value of $\mathcal{L}_{phy}$. 
It describes the average penetration depth over all simulation steps, all faces of reference mesh, and all source vertices. 

% \vpara{Comments/discussions on the collision response-baesd deformation proejction}
% Based on $\mathcal{L}_{proj}$, the projected deformation basis for each part is calculated via $$

\vpara{Total losses.} 
% for lossses at the training time, finetuning time, and inference time
At the pre-training stage, the basis prediction loss is added to train the basis prediction network, \emph{i.e.,} $\mathcal{L} = \mathcal{L}_{basis}$. 
At the fine-tuning stage, the total loss term is composed of the basis prediction loss, and the physical penalty term, \emph{i.e.,} $\mathcal{L} = \mathcal{L}_{basis} + \lambda_{phy}\mathcal{L}_{phy}$, where $\lambda_{phy}$ is a weight term empirically set to 1.0. 


\begin{algorithm}[H]
% \algsetup{linenosize=\tiny}
\small %\small, \footnotesize, \scriptsize, or \tiny
\caption{Single step collision avoidance. ``NONE\_MOTION'' indicates fixed parts. 
% denotes 
% the property of the fixed part. 
}
\label{algo_phy_sim_single_part_single_sim}
\footnotesize
    \begin{algorithmic}[1]
        \Require
            Part mesh 
            % Moving part mesh 
            $\mathcal{S}_{mov} = (\mathcal{V}_{mov}, \mathcal{E}_{mov})$ to articulate at the rest pose, reference part mesh $\mathcal{S}_{ref} = (\mathcal{V}_{ref}, \mathcal{E}_{ref})$, the number of simulation steps $N_{step}$, joint information $\mathcal{J}$, lower joint state $a$, upper joint state $b$. 
            % A set of convex bases $\{ \mathbf{B}_i \vert 1\le i\le C \}$, transformation coefficients $\{ \mathbf{A}_i \vert 1\le i\le C\}$, number of optimization iterations $T$. 
        \Ensure
            Average penetration depth APD/Collision penalty term $\mathcal{L}_{phy}$ and projection loss $\mathcal{L}_{proj}$ for the current part in this simulation process. 
        \If{$\mathcal{J}$.type == NONE\_MOTION}  \\ 
            \Return 0 , 0
        \EndIf
        \State $\mathcal{N}_{ref} \leftarrow \text{Face-Normal}(\mathcal{V}_{ref}, \mathcal{E}_{ref})$
        \State $\mathbf{d}^0 \leftarrow \text{Vertex-Face-Distance}(\mathcal{V}_{mov}, \mathcal{V}_{ref}, \mathcal{E}_{ref}, \mathcal{N}_{ref})$ % d_prev \in R^
        \State $\mathbf{S}^0 \leftarrow \text{Sign}(\mathbf{d}^0)$
        \State $\mathcal{D}\leftarrow \emptyset$
        \State $\mathcal{D}_{proj}\leftarrow \emptyset$
        \For{$t = 1$ to $N_{step}$}
            \State $s^t\leftarrow a + (b - a) \times t / N_{step}$
            \State $\mathcal{V}_{mov}^t\leftarrow \text{Articulation-Simulation}(\mathcal{V}_{mov}, s^t, \mathcal{J})$ % compute mov vertices
            \State $\mathbf{d}^t \leftarrow \text{Vertex-Face-Distance}(\mathcal{V}_{mov}^t, \mathcal{V}_{ref}, \mathcal{E}_{ref}, \mathcal{N}_{ref})$
            \State $\mathbf{S}^t \leftarrow \text{Sign}(\mathbf{d}^t)$
            \State $\mathbf{C}^t\leftarrow \text{Vertices-In-Faces}(\mathcal{V}_{mov}^t, \mathcal{V}_{ref}, \mathcal{E}_{ref})$
            \State $\mathbf{C}^t \leftarrow \mathbf{C}^t \wedge (\mathbf{S}^t \neq  \mathbf{S}^{t-1} )$
            \State ${d}^t \leftarrow \text{Mean}(\mathbf{C}^t \cdot \mathbf{d}^t \cdot \mathbf{S}^t )$
            \State $\mathcal{D} \leftarrow  \mathcal{D}  \cup \{  {d}^t\}$

            \State $\Delta \mathcal{V}_{mov}\leftarrow \mathcal{V}_{mov}^t - \mathcal{V}_{mov}^{t-1}$
            \State $d_{proj}^t\leftarrow \text{Mean}(\text{Sum}(\Delta \mathcal{V}_{mov} \cdot \mathbf{C}^t \cdot \mathbf{d}^t \cdot \mathcal{N}_{ref}))$
            \State $\mathcal{D}_{proj} \leftarrow  \mathcal{D}_{proj}  \cup \{  {d}_{proj}^t\}$
            
            
        \EndFor\\
        \State $\mathcal{L}_{phy}^{cur} \leftarrow \text{Mean}(\mathcal{D})$
        \State $\mathcal{L}_{proj}^{cur} \leftarrow \text{Mean}(\mathcal{D}_{proj})$ \\ 
        \Return $\mathcal{L}_{phy}^{cur}$ , $\mathcal{L}_{proj}^{cur}$
        
    \end{algorithmic}
\end{algorithm}


\begin{algorithm}[H]
% \algsetup{linenosize=\tiny}
\small %\small, \footnotesize, \scriptsize, or \tiny
\caption{Collision avoidance
}
\label{algo_phy_sim}
\footnotesize
    \begin{algorithmic}[1]
        \Require
            A set of part meshes $\{ \mathcal{S} = (\mathcal{V}, \mathcal{E}) \}$, a set of joint information $\{ \mathcal{J} \}$, a set of lower joint states $\{ a\}$, a set of upper joint state $b$. 
            Number of simulation steps $N_{step}$. Number of reference states for detection $N_{det}$. 
            % Part mesh 
            % Moving part mesh 
            % $\mathcal{S}_{mov} = (\mathcal{V}_{mov}, \mathcal{E}_{ref})$ to articulate at the rest pose, reference part mesh $\mathcal{S}_{ref} = (\mathcal{V}_{ref}, \mathcal{E}_{ref})$, number of simulation steps $N_{step}$, joint information $\mathcal{J}$, lower joint state $a$, upper joint state $b$. 
            % A set of convex bases $\{ \mathbf{B}_i \vert 1\le i\le C \}$, transformation coefficients $\{ \mathbf{A}_i \vert 1\le i\le C\}$, number of optimization iterations $T$. 
        \Ensure
            Average penetration depth APD/Collision penalty term $\mathcal{L}_{phy}$, Projection loss $\mathcal{L}_{proj}$. 
            
        \State $\mathcal{D}\leftarrow \emptyset$
        \State $\mathcal{D}_{proj}\leftarrow \emptyset$
        \For{$\mathcal{S}_{mov}\in \{ \mathcal{S} \} $}
            \For{$i_{step} = 1$ to $N_{det}$}
                \State Sample an articulation state for each part expect for $\mathcal{S}_{mov}$: $\{ s_{\mathcal{S}}  \vert \mathcal{S} \in \{ \mathcal{S} \}, \mathcal{S} \neq \mathcal{S}_{mov} \}$
                % \State $\{ \hat{\mathcal{S}} = \text{Articulation-Simulation}(\mathcal{S}, s_{\mathcal{S}}, \mathcal{J}_{\mathcal{S}}) \vert \mathcal{S}\in \{ \mathcal{S} \}, \mathcal{S} \neq \mathcal{S}_{mov} \}$
                \State Put parts except for $\mathcal{S}_{mov}$ into their sampled states; Put $\mathcal{S}_{mov}$ into the rest pose state. 
                % \State Put part shapes into a random sampled articulation state except for $\mathcal{S}_{mov}$
                \State $\mathcal{S}_{ref} \leftarrow \text{Merge-Meshes}(\{ \mathcal{S} \} \setminus \{ \mathcal{S}_{mov}\} )$
                \State  
                % \begin{equation*}
                %     s_{phy}^{cur}, s_{proj}^{cur} \leftarrow \\ 
                %     \text{Collision-Avoidance-Single-Step}(\mathcal{S}_{mov}, \mathcal{S}_{ref}, N_{step}, \mathcal{J}_{\mathcal{S}_{mov}}, a_{\mathcal{S}_{mov}}, b_{\mathcal{S}_{mov}})
                % \end{equation*}
                $s_{phy}^{cur}, s_{proj}^{cur} \leftarrow \text{Single-Step-Collision-Avoidance}(\mathcal{S}_{mov}, \mathcal{S}_{ref})$
                \State $\mathcal{D}_{phy} \leftarrow  \mathcal{D}_{phy}  \cup \{  s_{phy}^{cur}\}$
                \State $\mathcal{D}_{proj} \leftarrow  \mathcal{D}_{proj}  \cup \{  s_{proj}^{cur}\}$
            \EndFor
        \EndFor\\

        % \State $\mathcal{N}_{ref} \leftarrow \text{Face-Normal}(\mathcal{V}_{ref}, \mathcal{E}_{ref})$
        % \State $\mathbf{d}^0 \leftarrow \text{Vertex-Face-Distance}(\mathcal{V}_{mov}, \mathcal{V}_{ref}, \mathcal{E}_{ref}, \mathcal{N}_{ref})$ % d_prev \in R^
        % \State $\mathbf{S}^0 \leftarrow \text{Sign}(\mathbf{d}^0)$
        % \State $\mathcal{D}\leftarrow \emptyset$
        % \State $\mathcal{D}_{proj}\leftarrow \emptyset$
        % \For{$t = 1$ to $T$}
        %     \State $s^t\leftarrow a + (b - a) \times t / N_{step}$
        %     \State $\mathcal{V}_{mov}^t\leftarrow \text{Articulation-Simulation}(\mathcal{V}_{mov}, s^t, \mathcal{J})$ % compute mov vertices
        %     \State $\mathbf{d}^t \leftarrow \text{Vertex-Face-Distance}(\mathcal{V}_{mov}^t, \mathcal{V}_{ref}, \mathcal{E}_{ref}, \mathcal{N}_{ref})$
        %     \State $\mathbf{S}^t \leftarrow \text{Sign}(\mathbf{d}^t)$
        %     \State $\mathbf{C}^t\leftarrow \text{Vertices-In-Faces}(\mathcal{V}_{mov}^t, \mathcal{V}_{ref}, \mathcal{E}_{ref})$
        %     \State $\mathbf{C}^t \leftarrow \mathbf{C}^t \wedge (\mathbf{S}^t \neq  \mathbf{S}^{t-1} )$
        %     \State ${d}^t \leftarrow \text{Mean}(\mathbf{C}^t \cdot \mathbf{d}^t )$
        %     \State $\mathcal{D} \leftarrow  \mathcal{D}  \cup \{  {d}^t\}$

        %     \State $\Delta \mathcal{V}_{mov}\leftarrow \mathcal{V}_{mov}^t - \mathcal{V}_{mov}^{t-1}$
        %     \State $d_{proj}^t\leftarrow \text{Mean}(\text{Sum}(\Delta \mathcal{V}_{mov} \times \mathbf{C}^t \times \mathbf{d}^t \times \mathcal{N}_{ref}))$
        %     \State $\mathcal{D}_{proj} \leftarrow  \mathcal{D}_{proj}  \cup \{  {d}_{proj}^t\}$
            
            
        % \EndFor\\
        \State $\mathcal{L}_{phy} \leftarrow \text{Mean}(\mathcal{D})$
        \State $\mathcal{L}_{proj} \leftarrow \text{Mean}(\mathcal{D}_{proj})$ \\ 
        \Return $\mathcal{L}_{phy}$ , $\mathcal{L}_{proj}$
        
    \end{algorithmic}
\end{algorithm}


% \subsection{Collision response-based deformation projection}

% \subsection{Average penetration depth}



\subsection{Additional Explanations} \label{sec_supp_method_additional_details}


\vpara{Convex decomposition.} 
For rigid categories, we set the number of convexes to 256. 
For articulated objects, we list their settings in Table~\ref{tb_exp_convex_nn}. 
For each part, we first try the 128 convexes setting and double the number of convexes by 2 if BSP-Net's training loss cannot be converged. 

We draw some examples of decomposed convexes for the Table category in Figure~\ref{fig_table_cvx_decomposition} for an intuitive understanding. 

\begin{table*}[t]
    \centering
    \caption{\footnotesize 
    The number of convexes used for convex decomposition for each part of each articulated object category. 
    } 
    \begin{tabular}{@{\;}c@{\;}|c|c|c|c|c|c@{\;}}
    \midrule
        \hline
        \specialrule{0em}{1pt}{0pt} 
        Method & \makecell[c]{Storage\\ Furniture} & Scissors &  Eyeglasses  & Oven & Lamp & TrashCan \\ 
        \cline{1-7} 
        \specialrule{0em}{1pt}{0pt}
        
        Link 0 & 128 & 128 & 128 & 128 & 128 & 128 
        \\ \cline{1-7} 
        \specialrule{0em}{1pt}{0pt}

        Link 1 & 512 & 128 & 128 & 512 & 128 & 512 
        \\ \cline{1-7} 
        \specialrule{0em}{1pt}{0pt}

        Link 2 & 512 & - & 128 & - & 128 & - 
        \\ \cline{1-7} 
        \specialrule{0em}{1pt}{0pt}

         Link 3 & - & - & - & - & 128 & - 
        \\ \cline{1-7} 
        \specialrule{0em}{1pt}{0pt}

    \end{tabular}
    % }
    % \vspace{-16pt}
    \label{tb_exp_convex_nn}
\end{table*} 




\begin{figure*}[ht]
    \centering
    %   \includegraphics[width=0.85\textwidth]{./imgs/all-vis-17.pdf}
      \includegraphics[width=1.0\textwidth]{./figs/smooth_layer.pdf}
      % \vspace{-5pt}
    \caption{ \footnotesize
        The effectiveness of the mesh smooth layer for combining convex deformations. 
        For every three shapes, the leftmost one is the source shape for deformation, the middle one is the composed mesh without smoothing, and the right one is the smoothed shape. 
        }
    % }
    \label{fig_smooth_layer}
\end{figure*}

\vpara{Mesh smooth layer for combining multi-cage deformations.}
Usually, directly composing deformed convex shapes for the part mesh would lead to unwanted surfaces. To tackle this issue, we further add a smooth layer following~\cite{garcia2013cages} to change vertices interpolation weights, providing us with 
% leading us to 
smooth outputs. 
In Figure~\ref{fig_smooth_layer} we draw the deformation results before and after smoothing for a visual understanding of its effectiveness. 


\begin{figure*}[ht]
    \centering
    %   \includegraphics[width=0.85\textwidth]{./imgs/all-vis-17.pdf}
      \includegraphics[width=0.8\textwidth]{./figs/table-cvx-decompose.pdf}
      % \vspace{-5pt}
    \caption{ \footnotesize
        Examples for decomposed convexes (converted to point clouds) for the Table category. 
        Different colors represent different convexes. Notice the color bleeding artifact is just due to point cloud visualization while the convexes are just simple convex polyhedra.
        } 
    % }
    \label{fig_table_cvx_decomposition}
\end{figure*}
